# Supplementary material for: On the Validity of Consensus
Source: arXiv:2301.04920 source file (2023-06-26)
Supplement: Supplementary file 2 [file lower_bound_extended.tex]

\section{Lower Bound on Message Complexity for the ``Blockchain'' Validity Property} \label{section:blockchain_validity_appendix}

In this section, we show the quadratic lower bound on the message complexity for the ``blockchain'' validity property.
For the original formalism, the bound is shown for all validity properties in \Cref{subsection:lower_bound}.

The \emph{Blockchain Validity} is a validity property in which the input and output spaces are not known.
Recall the example of a blockchain system in which servers propose transactions issued by the clients.
Furthermore, for \emph{Blockchain Validity}, the discovery function is defined as (a subset of) all possible concatenations of the proposals.
For instance, $\mathsf{discover}\big( \{v_1, v_2\} \big) \subseteq \{v_1, v_2, v_1 || v_2, v_2 || v_1 \}$.

Let us fix a Byzantine consensus algorithm $\mathcal{A}$ with \emph{Blockchain Validity}.
By means of contradiction, let us assume that correct processes send $< (\frac{t}{2})^2$ messages in $\mathcal{E}_{\mathit{base}} \in \mathit{execs}(\mathcal{A})$; $\mathcal{E}_{\mathit{base}}$ is defined in \Cref{subsection:lower_bound}.
Then, by \Cref{lemma:behavior_without_receptions}, some correct process $Q$ has a behavior in which it decides some value $v \in \mathcal{V}_O$ without receiving any messages from other processes.
Moreover, due to the definition of the $\mathsf{discover}(\cdot)$ function, $v$ must be $Q$'s proposal in the aforementioned behavior.

Furthermore, in any canonical execution in which (1) $Q$ is faulty, and (2) no correct process proposes $v$, correct processes must decide some value $v' \neq v$ (due to the $\mathsf{discover}(\cdot)$ function).
Hence, by ``merging'' this execution with the behavior of $Q$ in which (1) $v$ is decided, and (2) no message (from other processes) is received, we reach disagreement.
Therefore, \emph{Blockchain Validity} requires quadratic number of messages to be exchanged by the correct processes.

\begin{theorem} [Lower bound on message complexity]
The message complexity of $\mathcal{A}$, which satisfies Blockchain Validity, is $\Omega(t^2)$.
\end{theorem}
