# Supplementary material for: On the Validity of Consensus
Source: arXiv:2301.04920 source file (2023-06-26)
Supplement: Supplementary file 3 [file necessary.tex]

\section{Necessary Conditions for Solvable Validity Properties: Formal Proof} \label{section:necessary_formal_proofs}

In this section, we give a formal proof that the similarity and knowledge conditions are necessary for a validity property to be solvable.
First, we start by showing that a ``common'' value must be decided in executions in which faulty processes do not take any computational steps.

\begin{lemma} \label{lemma:helper}
Let $\mathit{val}$ be any solvable validity property and let $\mathcal{A}$ be any partially synchronous algorithm which solves the Byzantine consensus problem with $\mathit{val}$.

Let $\mathcal{E} = (\mathcal{A}, c, \mathcal{F}, \epsilon, \text{GST})$ be any execution of $\mathcal{A}$ such that (1) $\epsilon$ is infinite, and (2) for every event $e \in \epsilon$, $e$ does not occur on any process $Q \in \mathcal{F}$.
Let $v \in \mathcal{V}$ be the decided value in $\mathcal{E}$.
Then, $v \in \bigcap\limits_{c' \in \mathit{sim}(c)} \mathit{val}(c')$.
\end{lemma}
\begin{proof}
By contradiction, suppose that $v \notin \bigcap\limits_{c' \in \mathit{sim}(c)} \mathit{val}(c')$.
Note that $\mathcal{F} \neq \emptyset$, as, otherwise, $v \in \bigcap\limits_{c' \in \mathit{sim}(c)} \mathit{val}(c')$ (given that $\mathit{sim}(c) = \{c\}$ in this case).

Let $c' \in \mathcal{I}$ be an input configuration such that (1) $c' \sim c$, and (2) $v \notin \mathit{val}(c')$.
We aim to construct an execution $\mathcal{E}'$ of $\mathcal{A}$ such that (1) $\mathcal{E}'$ corresponds to $c'$, and (2) $v \notin \mathit{val}(c')$ is decided in $\mathcal{E}'$.

Recall that $\process{c'} \cap \process{c} \neq \emptyset$ (by \Cref{definition:similarity_condition}); let $P$ be any process in $\process{c'} \cap \process{c}$.
We denote by $\epsilon_P$ the prefix of $\epsilon$ such that the last event of $\epsilon_P$ is $\big( P, \mathsf{decide}(v) \big)$ (given that $\epsilon$ is infinite and $\mathcal{A}$ solves the Byzantine consensus problem, $\big( P, \mathsf{decide}(v) \big) \in \epsilon$).
Let $T = \mathsf{time}((P, \mathsf{decide}(v)), \epsilon)$ be the time at which $P$ decides $v$ in $\epsilon$.
% We construct another sequence of events $\epsilon'$ in the following manner:
% \begin{compactenum}
%     \item $\epsilon' \gets \epsilon_P$.
    
%     \item For every process $Q \in \pi(c')$ such that $\big( Q, \mathsf{start} \big) \notin \epsilon_P$:
%     \begin{compactenum}
%         \item $\epsilon' \gets \epsilon' || \big( Q, \mathsf{start} \big)$.
%     \end{compactenum}
% \end{compactenum}
Finally, $\mathcal{E}' = (\mathcal{A}, c', \mathcal{F}' = \Pi \setminus{\process{c'}}, \epsilon' = \epsilon_P, \text{GST}' > T)$.
Moreover, for every event $e \in \epsilon'$, the following holds:
\begin{compactitem}
    \item If $e \in \epsilon_P$, then $\mathsf{time}(e, \epsilon') = \mathsf{time}(e, \epsilon)$.
    
    \item Otherwise, $\mathsf{time}(e, \epsilon') = T$.
\end{compactitem}

To conclude the proof, we show that $\mathcal{E}'$ satisfies the properties of an execution (see \Cref{section:full_model}):
\begin{compactenum}
    \item For every process $P \in \Pi$, $\epsilon'|_P$ is a behavior as (1) $\mathcal{E}$ satisfies this property, and (2) only the $\mathsf{start}$ events are appended to $\epsilon_P$.
    
    \item This property trivially holds as $\epsilon'$ is not infinite.
    
    \item For every process $P \in \pi(c) \cap \pi(c')$, the proposal of $P$ is identical in both $c$ and $c'$ (thus, in $\mathcal{E}$ and $\mathcal{E}'$).
    Moreover, for every process $Q \in \pi(c') \setminus{\pi(c)}$, only $\big( Q, \mathsf{start} \big)$ event belongs to $\epsilon'$.
    
    \item Due to the construction of $\mathcal{E}'$, $\mathsf{valid}(\mathcal{A}, P, \epsilon'|_P) = \mathit{true}$, for every process $P \in \Pi$.
    
    \item This property is satisfied since (1) it is satisfied by $\mathcal{E}$, and (2) only the $\mathsf{start}$ events are appended to $\epsilon_P$.
    
    \item This property is trivially satisfied as $\text{GST}' > \mathsf{time}( \epsilon'[|\epsilon'|], \epsilon')$.
    % by construction: every process $P \in \pi(c')$ starts by GST.
    
    \item This property trivially holds as $\epsilon'$ is not infinite.
    
    \item This property trivially holds for $\text{GST}' > T$ (i.e., GST is ``shifted'' to the future).
    
    \item This property trivially holds for $\text{GST}' > T$ (i.e., GST is ``shifted'' to the future).
\end{compactenum}
Hence, $\mathcal{E}'$ satisfies the properties introduced in \Cref{section:full_model}.
Therefore, $v \notin \mathit{val}(c')$ is decided in $\mathcal{E}'$.
We reach a contradiction with a fact that $\mathcal{A}$ solves the Byzantine consensus problem with $\mathit{val}$.
Thus, the lemma.
\end{proof}

Next, we give a formal proof that the similarity condition is necessary.
Recall that a validity property $\mathit{val}$ satisfies the similarity condition if and only if, for every input configuration $c \in \mathcal{I}$, $\bigcap\limits_{c' \in \mathit{sim}(c)} \mathit{val}(c') \neq \emptyset$ (by \Cref{definition:similarity_condition}). 

\begin{theorem}[The similarity condition is necessary]
If a validity property does not satisfy the similarity condition, the validity property is unsolvable.
\end{theorem}
\begin{proof}
By contradiction, assume that there exists a validity property $\mathit{val}$ such that (1) $\mathit{val}$ does not satisfy the similarity condition, and (2) $\mathit{val}$ is solvable.
Hence, there exists an algorithm $\mathcal{A}$ which solves the Byzantine consensus problem with $\mathit{val}$.
As $\mathit{val}$ does not satisfy the similarity condition, there exists an input configuration $c \in \mathcal{I}$ such that $\bigcap\limits_{c' \in \mathit{sim}(c)} \mathit{val}(c') = \emptyset$ (by \Cref{definition:similarity_condition}).
% Note that $\pi(c) \neq \Pi$ as, otherwise, $c$ would not ``violate'' the similarity condition given that $\mathit{sim}(c) = \{c\}$.

Let $\mathcal{E} = (\mathcal{A}, c, \mathcal{F} = \Pi \setminus{\pi(c)}, \epsilon, \text{GST})$ be an execution of $\mathcal{E}$ such that (1) $\epsilon$ is infinite, and (2) for every event $e \in \epsilon$, $e$ does not occur on any process $Q \in \mathcal{F}$.
Let $v \in \mathcal{V}$ be the decided value in $\mathcal{E}$.
By \Cref{lemma:helper}, $v \in \bigcap\limits_{c' \in \mathit{sim}(c)} \mathit{val}(c')$, which contradicts the fact that $\bigcap\limits_{c' \in \mathit{sim}(c)} \mathit{val}(c') = \emptyset$.
Thus, the theorem.
\end{proof}

Lastly, we show that the knowledge condition is a necessary condition for a validity property to be solvable.
Recall that a validity property $\mathit{val}$ satisfies the knowledge condition if and only if there exists a function $\Lambda: \mathcal{I} \to \mathcal{V}$ such that, for every input configuration $c \in \mathcal{I}$ where $|\process{c}| = n - t$, $\Lambda(c) \in \bigcap\limits_{c' \in \mathit{sim}(c)} \mathit{val}(c')$ (by \Cref{definition:knowledge_condition}).

\begin{theorem}[The knowledge condition is necessary]
If a validity property does not satisfy the knowledge condition, the validity property is unsolvable.
\end{theorem}
\begin{proof}
By contradiction, let there exist a validity property $\mathit{val}$ such that (1) $\mathit{val}$ does not satisfy the knowledge condition, and (2) there exists a partially synchronous algorithm $\mathcal{A}$ which solves the Byzantine consensus problem with $\mathit{val}$.
As $\mathit{val}$ does not satisfy the knowledge condition, there does not exist a function $\Lambda$ such that, for every input configuration $c \in \mathcal{I}$ where $|\process{c}| = n - t$, $\Lambda(c) \in \bigcap\limits_{c' \in \mathit{sim}(c)} \mathit{val}(c')$.

Fix any input configuration $c \in \mathcal{I}$ such that $|\pi(c)| = n - t$.
Consider exactly one execution $\mathcal{E}_c = (\mathcal{A}, c, \mathcal{F}_c, \epsilon_c, \text{GST}_c)$ of $\mathcal{A}$ such that (1) $\epsilon_c$ is infinite, and (2) for every event $e \in \epsilon_c$, $e$ does not occur on any process $Q \in \mathcal{F}_c$.
Let $v \in \mathcal{V}$ be the decided value in $\mathcal{E}_c$.
Due to \Cref{lemma:helper}, $v \in \bigcap\limits_{c' \in \mathit{sim}(c)} \mathit{val}(c')$.
Hence, $\Lambda(c)$ is defined: $\Lambda(c)$ is the decision value of $\mathcal{E}_c$.

Given that the aforementioned argument can be applied to any input configuration $c \in \mathcal{I}$ with $|\process{c}| = n - t$, the $\Lambda$ function satisfying \Cref{definition:knowledge_condition} exists.
Therefore, we reach a contradiction with the fact that the $\Lambda$ function does not exist.
Thus, the theorem.
\end{proof}
